# Supplementary material for: Machine Learning LSST 3x2pt analyses -- forecasting the impact of systematics on cosmological constraints using neural networks
Source: arXiv:2403.11797 source file (2024-03-18)
Supplement: Supplementary file 1 [file emu_test.tex]

\section{Emulator accuracy for impact studies}\label{app:emu_accuracy}

\begin{figure}
    \centering
    \includegraphics[width=\linewidth]{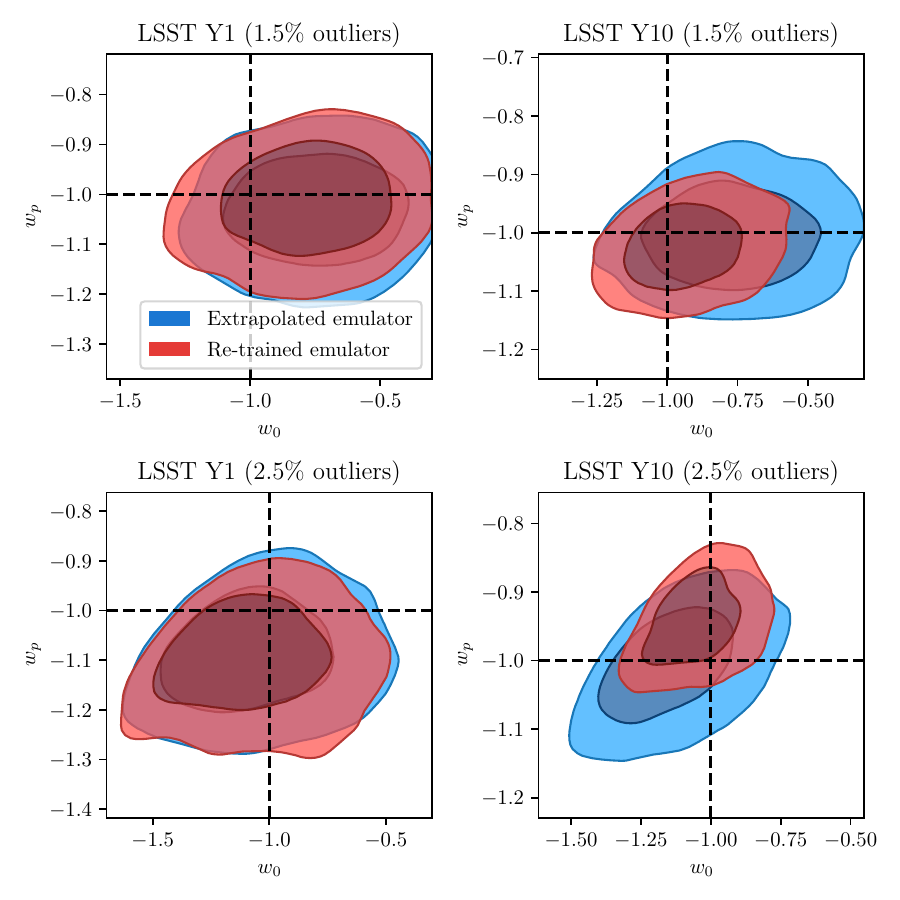}
    \caption{The constraints on $w_0$-$w_p$ parameters when using an emulator outside its training region (blue contours) and when we retrain the emulator with training points in its high posterior region (red contours). Different rows shows the shows the analysis of data vectors with different fractions of photo-$z$ outliers as indicated in the title. The left (right) columns shows the results for LSST-Y1 (Y10) analysis choices. As we can see, extrapolating the emulator does not give significantly different constraints for LSST-Y1 case, whereas the extrapolation leads to very different constraints for LSST-Y10 analysis choices.}
    \label{fig:emu_comparison}
\end{figure}

In sections \ref{sec:small_scales} and \ref{sec:photoz_outliers}, we used the emulator for impact studies, where the resulting posteriors are biased. Since our emulators are trained locally, using the emulators for parameter regions outside its training range requires extrapolation. As such, the emulator may not be reliable in these parameter regions and needs to be tested. 

Therefore, in this section, we test the accuracy of the emulators used in this paper for impact studies. Specifically, we reanalyze the results obtained in section \ref{sec:photoz_outliers} by re-training the emulator with the contaminated data vector so that they are now designed to obtain accurate posteriors for biased cosmological constraints. We train the emulators for analyzing the contaminated data vectors with 4 different photo-$z$ outlier fractions -- $1\%, 1.5\%, 2.5\%$ and $3 \%$. As in section \ref{sec:photoz_outliers}, we still analyze the data vectors assuming $2\%$ photo-$z$ outliers in the model. 

The results of these tests for the impact studies with $1.5\%$ and $2.5\%$ outlier fractions in the data vectors with LSST-Y1 and Y10 survey assumptions are shown in Figure \ref{fig:emu_comparison}. In that figure, the blue contours show the results obtained from the original emulator that is extrapolated to different region of the parameter space and the red contours show the results with the re-trained emulator. As we can see from the figure, the extrapolated emulator gives accurate results for the LSST-Y1 survey, whereas the results for LSST-Y10 are significantly different. Specifically, the uncertainty in the $w_0$-$w_p$ parameters are very different when the constraints are obtained properly. \red{(Cite Evan's paper)}
